# Supplementary material for: Prompt to Transfer: Sim-to-Real Transfer for Traffic Signal Control with Prompt Learning
Source: arXiv:2308.14284 source file (2024-01-20)
Supplement: Supplementary file 1 [file appendix.tex]

\appendix
% \paragraph{Appendix}

% Any appendices must appear after the main content. If your main sections are numbered, appendix sections must use letters instead of arabic numerals.

\section{Metrics for Traffic Signal Control} 

This paper follows the literature in TSC~\cite{zhao2011computational, wei2021recent}, and adopts commonly used traffic signal control metrics, a detailed description as below: \\
$\bullet$ \textit{Average Travel Time (ATT)} is the average time $t$ it takes for a vehicle to travel through a specific section of a road network. For a control policy, the smaller $ATT$, the better. \\
$\bullet$ \textit{Throughput (TP)} is the number of vehicles that have reached their destinations in a given amount of time. The larger $TP$, the better.\\
$\bullet$ \textit{Reward} is an RL term that measures the return by taking action $a_t$ under state $s_t$. We use the total number of waiting vehicles as the reward. The larger reward, the fewer waiting vehicles, the better.\\
$\bullet$ \textit{Queue} is the number of vehicles waiting to pass through a certain intersection in the road network. The smaller queue, the better.\\
$\bullet$ \textit{Delay} is the average delay per vehicle in seconds and measures the amount of time that a vehicle spends waiting in the network. The smaller delay, the better.

% \paragraph{B. DQN update process} 

\section{Full Correlation Analysis}
In this part, we provide a more complete version of correlation analysis in line with case study in Section~\ref{casestudy}. The values of $\Delta_{\text{Accuracy↑}}$, $\Delta_{\text{ATT↑}}$, $\Delta_{\text{TP↑}}$, $\Delta_{\text{Queue↑}}$ indicating how much gap is mitigated, they are further definitions based on Equation~\eqref{eq:delta}:
\begin{equation}\label{eq:gapimprove}
    \Delta_{\text{↑}} = \lvert \psi_{a\Delta} - \psi_{b\Delta} \rvert
\end{equation}
where $a$ and $b$ are two approaches used, here they are Vanilla-GAT and \ours, respectively. Based on the absolute value of this equation, since the \ours performs consistently better than Vanillia-GAT from \ref{tab:result}, the larger value $\Delta_{\text{↑}} $ is, the much more gap is mitigated. And since every metric has its own range, for unity, we normalized the $\Delta_{\text{↑}}$ using max-min normalization. Apart from the commonly used metrics, the $\Delta_{\text{Accuracy↑}}$ refers to how much accuracy (loss) has been improved. 

The results are shown in Figure~\ref{fig:correlation}. We could observe that, for the relation between the accuracy improvement $\Delta_{\text{Accuracy↑}}$ and each of the metrics, they are strongly correlated except for minor outlier points, which proves that, when the \ours provides a better depiction inference on the system dynamics, the inverse model's action would be better grounded to the realistic scenario, policy $\pi$ will learn in a more robust way and leading to a final lower performance gap in reality. Other metrics' mutual comparison also reflects the correctness of our method by showing a strong correlation between each other.
% \begin{figure}[h!]
%     \centering
%     \includegraphics[width=0.5\textwidth]{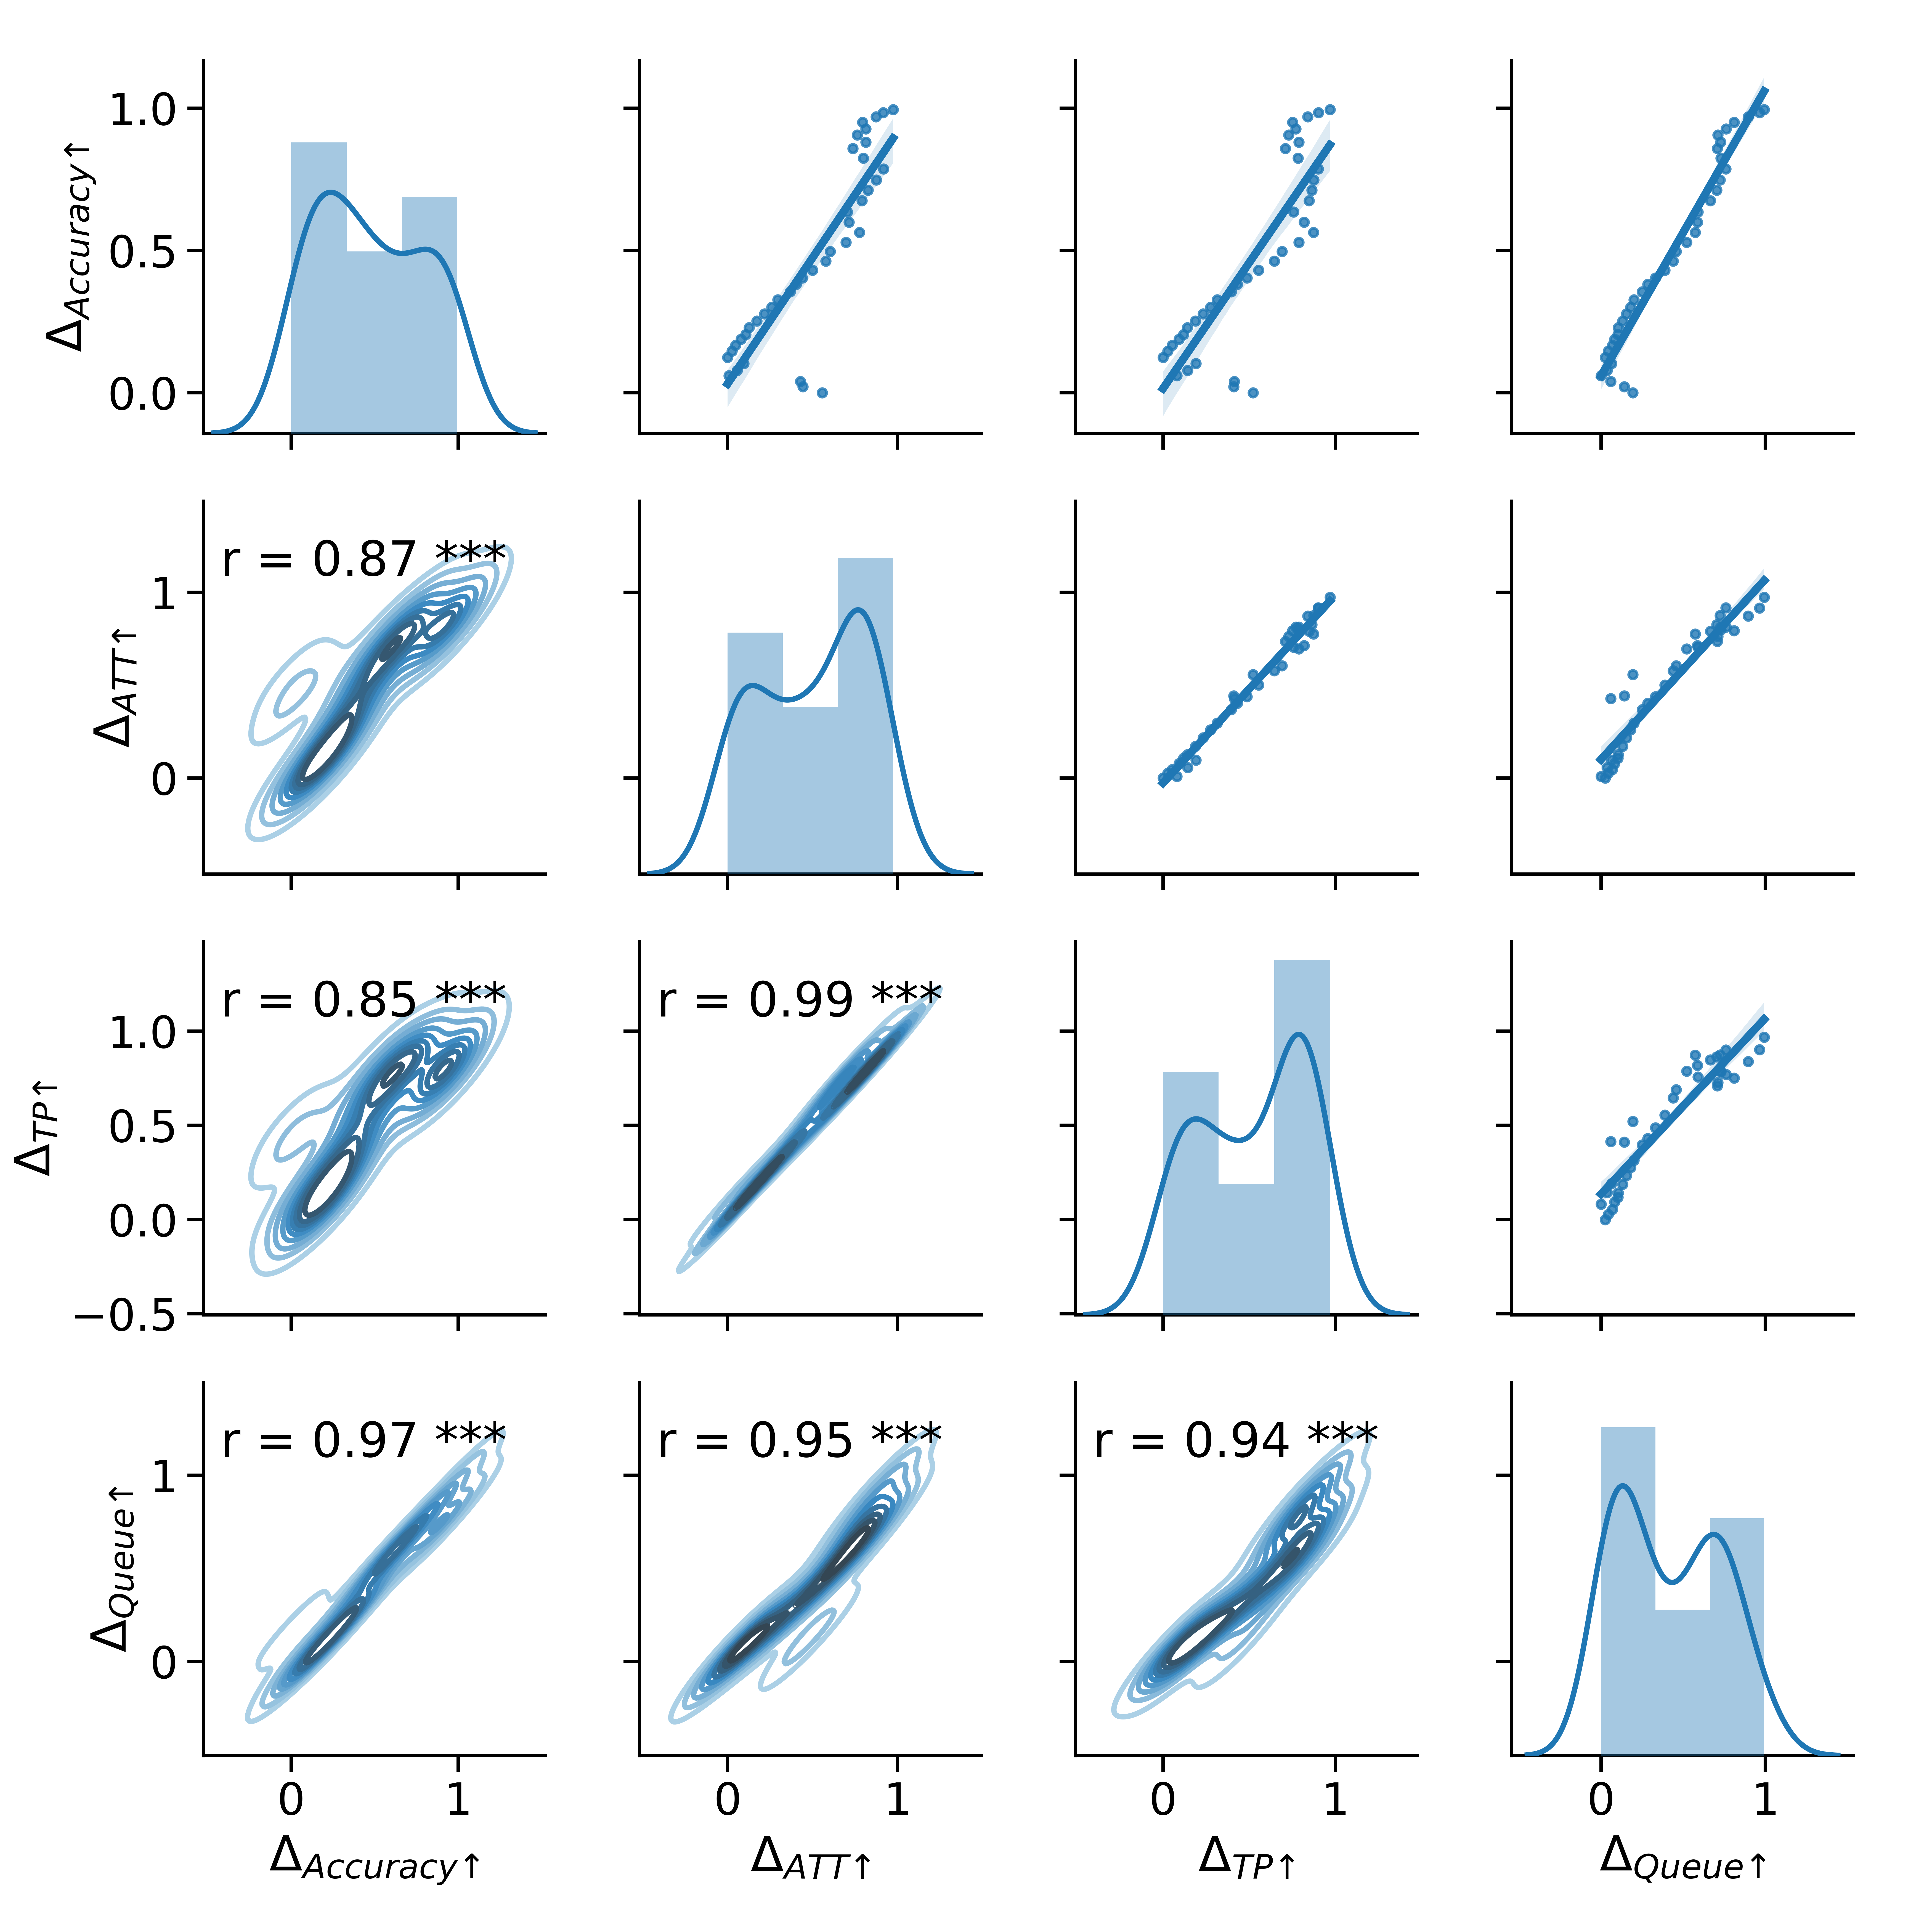}
%     \caption{Correlation analysis between improvements of forward model accuracy (compared with Vanilla-GAT) and the improvements of
% performance in $E_{real}$. The value of $r$
% indicates the Pearson Correlation Coefficient, and the values
% with $\ast$ indicating statistical significance for correlation, where
% $\ast\ast\ast$ indicates the p-value for testing non-correlation $p \leq$  0.001.}
%     \label{fig:correlation}
% \end{figure}

\section{Details of Prompt and Hyper-parameters}
In this part, we provide prompt templates and cases examples, as well as details of parameter settings in our experiment.

\paragraph{Prompt Examples}
First, we provide a chain-of-thought prompt example to understand how the LLM think given the scenario and inference target, so as to make sure the inference logic is correct according to human knowledge, we  prompt a question given the description below (green box):  \\
\begin{figure}[h!]
    \centering
    \includegraphics[width=0.5\textwidth]{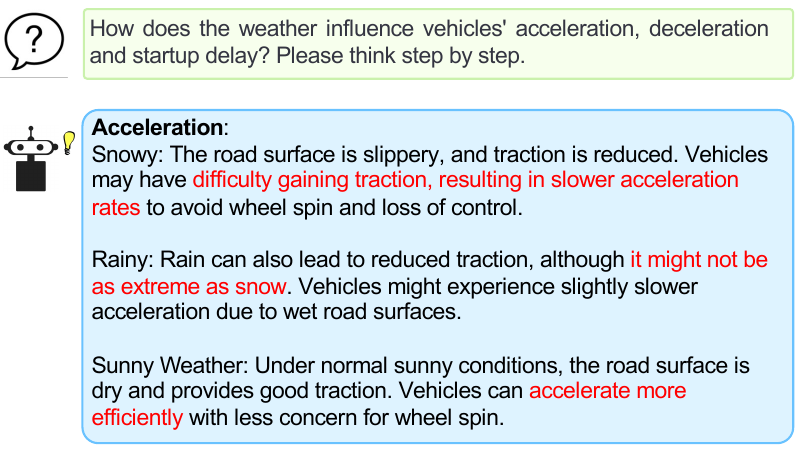}
    % \caption{}
    \label{fig:example1}
\end{figure}
\begin{figure}[h!]
    \centering
    \includegraphics[width=0.5\textwidth]{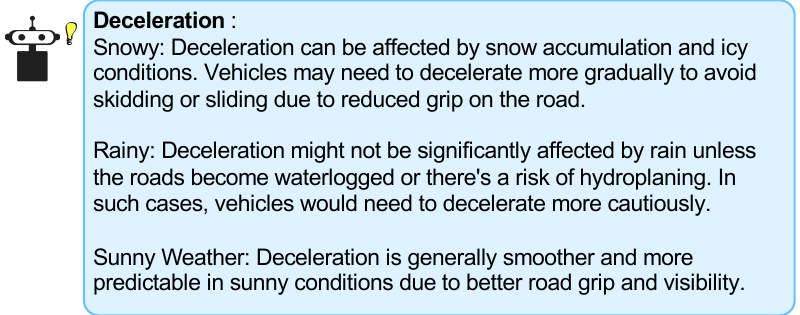}
    % \caption{}
    \label{fig:example2}
\end{figure}
\begin{figure}[h!]
    \centering
    \includegraphics[width=0.48\textwidth]{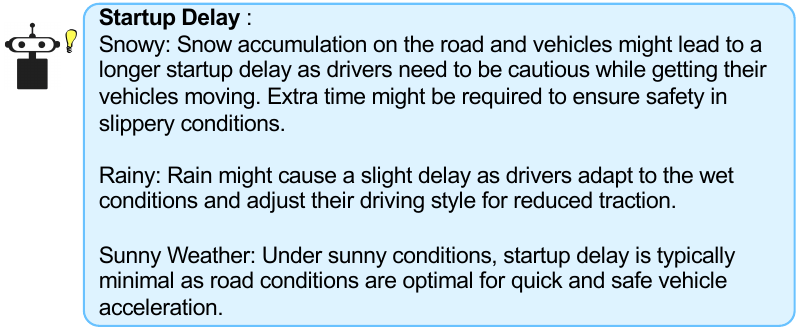}
    % \caption{}
    \label{fig:example3}
\end{figure}
% \vspace{-3mm}
We could notice that the thinking process is making sense and also considering the hieratical results based on extreme-level of weather conditions, the snowy weather would affect more than light rainy ones.
And the conclusion from LLM is:
\begin{tcolorbox}[colback=white!5,%gray background
                  colframe=black,% black frame colour
                  width=8.5cm,% Use 8cm total width,
                  arc=1mm, auto outer arc,
                  boxrule=0.35pt,
                  fontupper=\small, % Set font size to \small
                 ]
It's important to note that the influence of weather on vehicles' acceleration, deceleration, and startup delay can vary based on factors such as the type of vehicle, road conditions, driver behavior, and the severity of the weather. 
\end{tcolorbox}
Based on the explainable reasoning, we further provide the lane level traffic state - vehicle number to provide sufficient perceptible information for LLMs to make inferences. And incorporate into \ours as interpreted in Figure~\ref{fig:fuison}. In our setting, an LLM will be used to query on every lane state, the results are proven to be promising, however, the economic cost by requesting the LLM API is high, an alternative using a self-trained domain large model or other well-performed open-source models, which is to be explored in the future.

\paragraph{Hyper-parameters and set up with LibSignal}

Our experiment and code are based on LibSignal, an open-source library for traffic signal control tasks that incorporates multiple simulation
environments, providing a suitable testbed for sim-to-real performance. We first provide the parameter details and then introduce how we setup in LibSignal.

\begin{itemize}
\item Hyper-parameters: 
The World is a module controlling the common setting for various worlds like SUMO or Cityflow as in Table~\ref{tab:world}:  

\begin{table}[h!]
    \centering
    \caption{Parameters for world in LibSignal}
    \scalebox{1.}{
    \begin{tabular}{ccc}
        \toprule
        World & Item & Value \\ \midrule
         - & Seed & 0 \\
         - & Interval & 1.0 \\
         - & rlTrafficLight & True \\
        \bottomrule
    \end{tabular}}\label{tab:world}
\end{table}

Then we have defined parameters for the sim-to-real trainer which is responsible for policy training control and updating procedures. The params are provided below in Table~\ref{tab:trainer}.
\begin{table}[h!]
    \centering
    \caption{Parameters for sim-2-real trainer}
    \scalebox{1.}{
    \begin{tabular}{cc}
        \toprule
         Item & Value \\ \midrule
          learning\_start & 5000 \\
          buffer\_size & 5000 \\
          steps $T$& 3600 \\
          test\_steps & 3600 \\
          yellow\_length & 5 \\
          action\_interval & 10 \\
          episodes $I$& 300 \\
          update\_model\_rate & 1 \\
          update\_target\_rate & 5 \\
        \bottomrule
    \end{tabular}}\label{tab:trainer}
\end{table}
As for the DQN RL policy model, we have the following parameters in Table~\ref{tab:model}. And the Grounded action transformation models parameters are shared in Table~\ref{tab:GAT}. The model structure of the forward and the inverse model are released in the supplementary materials zip file of code. Which is defined in file `stat\_utils.py' file under the path of `Prompt\_GAT/common', `N\_net' class: forward model, and `N\_net\_back' class: inverse model. 

\begin{table}[h!]
    \centering
    \caption{Parameters for DQN RL-policy model}
    \scalebox{1.}{
    \begin{tabular}{cc}
        \toprule
         Item & Value \\ \midrule
         learning\_rate (lr) & 0.001 \\
          batch\_size & 64 \\
          gamma & 0.98 \\
          epsilon & 0.1 \\
          epsilon\_decay & 0.99 \\
          epsilon\_min & 0.01 \\
          grad\_clip & 0.5 \\
          one hot & True \\
        \bottomrule
    \end{tabular}}\label{tab:model}
\end{table}

\begin{table}[h!]
    \centering
    \caption{Parameters for \ours module}
    \scalebox{0.8}{
    \begin{tabular}{ccc}
        \toprule
         Item & Value & Explanation \\ \midrule
          pre\_train epoch $E$& 100 & Epochs pre-trained before action grounding\\
          forward epoch $n$& 20 & For the forward model per ground training \\ 
          inverse epoch $n$& 20 & For the inverse model\\
          forward lr & 1e-4 & learning rate for forward model\\ 
          inverse lr\_decay & 1e-5 & learning rate for inverse model\\
          batch\_size & 64 & same for both models \\
          % batch\_size & 0.5 \\
        \bottomrule
    \end{tabular}}\label{tab:GAT}
\end{table}

\item Set up with LibSignal: In LibSignal, we can easily customize our training script using any supported engines, which we take $\textit{SUMO}$ as $E_{{real}}$ and $\textit{CityFlow}$ as $E_{sim}$. In our code, we define a sim2real.py as the starting script for training, which calls a sim2real\_trainer.py and initializes the sim2realtask to register a trainer. In the trainer file, we define how to create worlds (simulators), what metrics to be used, and the agent to apply in interaction, then in the execution of the trainer, we define the inverse and forward models, and how to update policy networks.  In the `sim\_train' function under trainer, we apply the prompt process by introducing a function `query\_path\_condition', which takes query (traffic state, weather condition) as input, and constructs content based on a prompt template to interact with LLMs, with the returned answer, the extended observation will be used for dynamics profiling and forward model training, and help the policy to ground and take actions on a more realistic system dynamics.

\end{itemize}
